# Supplementary material for: Efficient Signature-Free Validated Agreement
Source: arXiv:2403.08374 source file (2024-08-20)
Supplement: Supplementary file 1 [file graded_consensus.tex]

% \section{Graded Consensus: Implementation \& Proof} \label{section:gccool}

This section focuses on graded consensus, the first building block of \name. 
Namely, we present its implementation (\Cref{subsection:gccool_algorithm}), and prove its correctness and complexity (\Cref{subsection:informal_analysis}).
% Formal proofs can be found in the full version of the paper~\cite{extended_version}.
% An analysis of the good (common) case can be found in \Cref{appendix:best_case}.

\subsection{Implementation} \label{subsection:gccool_algorithm}

Our implementation of the graded consensus primitive is given in \Cref{algorithm:gccool_protocol}.
\Cref{algorithm:gccool_protocol} leverages a binary graded consensus (using implementation proposed from \cite{Lenzen2022}) and \reducecool (\Cref{algorithm:reducecool}).
%Importantly, the binary graded consensus from \cite{Lenzen2022} satisfies an additional property:
% \begin{compactitem}
%     \item \emph{Safety:} If any correct process decides a pair $(\mathit{v}', \cdot)$, then $\mathit{v}'$ has been proposed by a correct process.
% \end{compactitem}
% \ayaz{I mentioned this property because it is currently used in some of the proofs. Technically, in a binary graded consensus (doesn't have to be by \cite{Lenzen2022}), this property is implied by the strong validity property}
\reducecool itself is a sub-protocol corresponding to the first part of the \textsc{COOL} protocol introduced by Chen~\cite{Chen2021}.
(\textsc{COOL} protocol is an error-free Byzantine agreement algorithm that satisfies \emph{only} strong validity and achieves $O\big( nL + n^2 \log(n) \big)$ bit complexity.)
% \gccool's pseudocode is given in \Cref{algorithm:gccool_protocol}.
% \gccool leverages \reducecool (\Cref{algorithm:gccool_protocol}), a sub-protocol corresponding to the first part of the \textsc{COOL} protocol \cite{Chen2021}.
Intuitively, \reducecool reduces the number of candidate outputs to at most 1; if all processes start with the same input value, that value is preserved by \reducecool.
% , while a unanimous inp will be necessarily preserved. 
Moreover, the processes output a binary success indicator from \reducecool. 
Again, a unanimous proposal leads to a common positive success indicator (i.e., $1$). 
Moreover, if a correct process outputs a positive success indicator (i.e., $1$), it is guaranteed that all correct processes agreed on a common value proposed by some correct process.

\begin{algorithm} [h]
\caption{Graded consensus: Pseudocode (for process $p_i$)}
\label{algorithm:gccool_protocol}
\begin{algorithmic} [1]
\footnotesize
    \State \textbf{Uses:}
    \State \reducecool~\cite{Chen2021}, \textbf{instance} $\mathcal{R}_{\mathit{cool}}$ \BlueComment{exchanged bits: $O\big(nL + n^2\log(n) \big)$; rounds: $5 \in O(1)$}
    \State Graded consensus proposed in~\cite{Lenzen2022}, \textbf{instance} $\mathcal{GC}$ \BlueComment{exchanged bits: $O(n^2)$; rounds: $2 \in O(1)$}

\medskip
\State Let $\omega_i$ denote $p_i$'s proposal.
%\State Let $(\omega^{(i)}, v_i, s_i, S_1) \in \mathsf{Value} \times \{0, 1\} \times \{0, 1\} \times (\text{set of processes})$ be a $p_i$'s local variable.
\State Let $(\omega^{(i)}, v_i) \in \mathsf{Value} \times \{0, 1\}$ be a $p_i$'s local variable.
\State Let $\mathit{decided}_i \in \{\mathit{true}, \mathit{false}\}$ be a $p_i$'s local variable initialized to $\mathit{false}$.

\medskip 
\State Let $(\omega^{(i)}, v_i) \gets \mathcal{R}_{\mathit{cool}}(\omega_i)$ \label{line:invoke_reduce} \BlueComment{\cite{Chen2021} ensures that if $(\omega^{(i)}, 1)$ is returned, then all correct processes return $(\omega_i, \cdot)$}% $|\{\omega^{(i)} | \omega^{(i)} \ne \phi \text{ and } p_i \text{ is correct}\}| \leq 1$}
% \State Let $(\omega^{(i)}, v_i, s_i, S_1) \gets \mathcal{R}_{\mathit{cool}}(\omega_i)$ \label{line:invoke_reduce} \BlueComment{\cite{Chen2021} ensures $|\{\omega^{(i)} | \omega^{(i)} \ne \phi \text{ and } p_i \text{ is correct}\}| \leq 1$}

\State Let $(b_i,g_i) \gets \mathcal{GC}(v_i)$ \label{line:invoke_graded_consensus} \BlueComment{if $\mathcal{GC}$ decides $(b, \cdot)$, then $b$ was proposed by a correct process}
\State \textbf{if} $b_i = 0$: \label{line:sad}
\State \hskip2em $p_i$ decides $(\omega_i, 0)$ \label{line:decide_1_its} \BlueComment{no correct process decides $(\omega \neq \omega_i, 1)$ from \Cref{algorithm:gccool_protocol}}
%\State \hskip2em $\mathit{decided}_i \gets \mathit{true}$

\State \textbf{if} $b_i = 1$: \label{line:happy}
\State \hskip2em $p_i$ decides $(\omega^{(i)}, g_i)$ \label{line:decide_2_its} 
%\State \hskip2em $\mathit{decided}_i \gets \mathit{true}$

% \medskip
% \State \textbf{Reconstruction phase:}

% \State \textbf{if} $\omega^{(i)} \neq \phi$:
% \State \hskip2em Let $[y_1^{(i)}, y_2^{(i)}, ..., y_n^{(i)}] \gets \mathsf{RSEnc}(\omega^{(i)}, n, k)$, where $k = \lfloor \frac{t}{5} \rfloor + 1$.
% \State \hskip2em $p_i$ sends $\langle y_j^{(i)} \rangle$ to every process $p_j$
% \label{line:send_help_symbols}

% \State \textbf{if} $s_i = 0$:
% \State \hskip2em $y_i^{(i)} \gets \mathsf{majority}(\{y_i^{(j)}, \text{for every process } p_j \in S_1\})$ \label{line:majority}
% \State $p_i$ broadcasts $\langle y_i^{(i)} \rangle$ \label{line:share_symbol}

% \State \textbf{if} $\mathit{decided}_i = \mathit{false}$:\label{line:check_decided}
% \State \hskip2em \LineComment{if $p_i$ does not receive an RS symbol from a process, it associates that process with any specific RS symbol}
% \State \hskip2em $p_i$ decides $(\mathsf{RSDec}(k, t, \text{received symbols}), g_i)$ \label{line:decide_3_its} \BlueComment{$p_i$ receives RS symbols from all processes} 

\end{algorithmic}
\end{algorithm}

\begin{algorithm} [hp]
\caption{\reducecool~\cite{Chen2021}: Pseudocode (for process $p_i$)}
\label{algorithm:reducecool}
\begin{algorithmic} [1]
\footnotesize
\State Set $\omega^{(i)} = w_i$. \BlueComment{Value $w_i$ is the proposal of process $p_i$.}
\State Process $p_i$ encodes its message into $n$ symbols, i.e., $[y_1^{(i)}, y_2^{(i)}, ..., y_n^{i}] \gets \mathsf{RSEnc}(w_i, n, k)$, where $k = \lfloor \frac{t}{5} \rfloor + 1$.
% as $y^{(i)}_j \triangleq h_{T_j} w_i$, $j \in [1 : n]$.

\medskip
\State \textbf{Phase 1:}
\State Process $p_i$ sends $(y^{(i)}_j , y^{(i)}_i)$ to process $p_j$, $\forall j \in [1 , n]$.
\For{$j = 1 \text{ to } n$}
    \If{$\big( (y^{(j)}_i , y^{(j)}_j) = (y^{(i)}_i , y^{(i)}_j) \big)$}
        \State Process $p_i$ sets $u_i(j) \gets 1$.
    \Else
        \State Process $p_i$ sets $u_i(j) \gets 0$.
    \EndIf
    \EndFor
    \If{$\left(\sum_{j=1}^{n} u_i(j) \geq n - t\right)$}
        \State Process $p_i$ sets its success indicator as $s_i \gets 1$.
    \Else
        \State Process $p_i$ sets $s_i \gets 0$ and $\omega^{(i)} \gets \phi$.
    \EndIf

\State Process $p_i$ sends the value of $s_i$ to all processes.
\State Process $p_i$ creates sets $S_p \gets \{j : s_j = p, j \in [1 : n]\}$, $p \in \{0, 1\}$, from received $\{s_j\}_{j=1}^{n}$.

\medskip
\State \textbf{Phase 2:}
\If{$(s_i = 1)$}
    \State Process $p_i$ sets $u_i(j) \gets 0$, $\forall j \in S_0$.
    \If{$\left(\sum_{j=1}^{n} u_i(j) < n - t\right)$}
        \State Process $p_i$ sets $s_i \gets 0$ and $\omega^{(i)} \gets \phi$.
    
    \State Process $p_i$ sends the value of $s_i$ to all processes.
    \EndIf
    \EndIf
    \State Process $p_i$ updates $S_0$ and $S_1$ based on the newly received success indicators.

\medskip
\State \textbf{Phase 3:}
\If{$(s_i = 1)$}
    \State Process $i$ sets $u_i(j) \gets 0$, $\forall j \in S_0$.
    \If{$\left(\sum_{j=1}^{n} u_i(j) < n - t\right)$}
        \State Process $p_i$ sets $s_i \gets 0$ and $\omega^{(i)} \gets \phi$.
    
    \State Process $p_i$ sends the value of $s_i$ to all processes.
    \EndIf
    \EndIf
    
    \State Process $p_i$ updates $S_0$ and $S_1$ based on the newly received success indicators.
    \State Process $p_i$ sends $\langle \textsc{symbol}, y_j^{(i)} \rangle$ to process $p_j$, $\forall j \in [1, n]$.
    \If{$\left(|S_1| \geq 2t + 1\right)$} \label{line:reduce_cool_S1geq2tp1}
        \State Process $p_i$ sets the binary vote as $v_i = 1$.
    \Else
        \State Process $p_i$ sets the binary vote as $v_i = 0$.
    \EndIf

\medskip
\State \textbf{Phase 4:}
\If{$s_i = 1$}
    \State Process $p_i$ sends $\langle \textsc{reconstruct}, y_i^{(i)} \rangle$ to all processes. \label{line:reduce_cool_bcast_reconstruct_1}
\Else
    \State Let $y_i^{(i)} \gets \mathsf{majority}(\text{RS symbols received via \textsc{symbol} messages})$. \label{line:majority}
    \State Process $p_i$ sends $\langle \textsc{reconstruct}, y_i^{(i)} \rangle$ to all processes. \label{line:reduce_cool_bcast_reconstruct_2}
\EndIf

\smallskip
\If{$s_i = 1$}
    \State \textbf{return} $(\omega^{(i)}, v_i)$ \label{line:reduce_cool_decide_1_its}
\Else  
    \State \textbf{return} $( \mathsf{RSDec}(k, t, \text{RS symbols received via \textsc{reconstruct} messages}), v_i )$ \label{line:reduce_cool_decide_2_its}
\EndIf

% \State \textbf{return} $(\omega^{(i)}, v_i, s_i, S_1)$     

\end{algorithmic}
\end{algorithm}

%%%%%%%%%%%%%%%%%%%%%%%%%%%%%%%%%%%%%%%%%%
%% end reduce sync COOL w/ O(f) latency %%
%%%%%%%%%%%%%%%%%%%%%%%%%%%%%%%%%%%%%%%%%%

\subsection{Proof of Correctness \& Complexity} \label{subsection:informal_analysis}

The following lemma states the properties ensured by the \reducecool protocol (\Cref{algorithm:reducecool}), proven in \cite{Chen2021}.
%The following lemma states some key intermediate results of~\cite{Chen2021} associated with the \reducecool protocol (\Cref{algorithm:reducecool}).
We emphasize that \reducecool utilizes a special value $\phi$.

\begin{lemma} \label{lemma:crucial_long_inputs}
All correct processes eventually output from the \reducecool protocol (termination of \reducecool).
Let $(\omega^{(i)}_{\mathit{proposal}}, v_i)$  %$(\omega^{(i)}_{\mathit{proposal}}, s_i, v_i, S_1^{(i)})$ 
denote the output received by a correct process $p_i$.
The following is guaranteed:
\begin{compactitem}
    \item Safety: If $\omega^{(i)}_{\mathit{proposal}} \neq \phi$, then $\omega^{(i)}_{\mathit{proposal}}$ is the value proposed by $p_i$ to \reducecool.

    \item Consistency: If there exists a correct process $p_i$ such that $v_i = 1$, then there exists a value $\omega$ such that every correct process receives $(\omega, \cdot)$ \label{item:consistency}

    % \item Non-duplicity: If there exists a correct process $p_i$ such that $v_i = 1$, then $|\{\omega^{(j)}_{\mathit{proposal}} \,|\, \omega^{(j)}_{\mathit{proposal}} \neq \phi \text{ and } p_j \text{ is correct} \}| \leq 1$. \label{item:non_duplicity}

    % \item Retrievability: If there exists a correct process $p_i$ such that $v_i = 1$, then $| \{ p_j | p_j \text{ is correct and } p_j \in S_1^{(i)} \text{ and }  \omega^{(j)}_{\mathit{proposal}} \neq \phi  \}| \geq t + 1$. \label{item:retrievability}

    \item Obligation: If every correct process proposes the same value $\bar{w}$, then every correct process receives $(\bar{w}, 1)$ from \reducecool. %$(\bar{w}, 1, 1, \cdot)$ from \reducecool. 
    \label{item:obligation}
\end{compactitem}
\end{lemma}
\begin{proof}
The proof of the lemma comes directly from the extended version~\cite{Chen2021extended} of~\cite{Chen2021}:
\begin{compactitem}
    \item Termination is ensured by~\cite[Lemma 6]{Chen2021extended}.
    \item Safety is ensured as $p_i$ never updates its variable to any other non-$\phi$ value (see \Cref{algorithm:reducecool}).

    \item Obligation is ensured by \cite[Lemma 5 (appendix H)]{Chen2021extended}.

    \item Consistency is ensured by \cite[Lemma 3]{Chen2021extended} and \cite[Lemma 4 (appendix G, equations 130 to 133)]{Chen2021extended}.
    More precisely,  \cite[Lemma 3]{Chen2021extended} ensures:
    \begin{compactitem}
    \item Non-Duplicity: If there exists a correct process $p_i$ such that, at the end of Phase 3 of the \reducecool protocol (\Cref{algorithm:reducecool}), $v_i = 1$, then 
    
    $|\{\omega^{(j)}_{\mathit{proposal}} \,|\, \omega^{(j)}_{\mathit{proposal}} \neq \phi \text{ at the end of \Cref{algorithm:reducecool} and } p_j \text{ is correct} \}| \leq 1$. \label{item:non_duplicity}
    \end{compactitem}
    While \cite[Lemma 4 (appendix G, equations 130 to 133)]{Chen2021extended} ensures
    \begin{compactitem}
    \item Retrievability: If there exists a correct process $p_i$ such that, at the end of Phase 3 of the \reducecool protocol (\Cref{algorithm:reducecool}), $v_i = 1$, then $| \{ p_j | p_j \text{ is correct and } p_j \in S_1^{(i)} \text{ and }  \omega^{(j)}_{\mathit{proposal}} \neq \phi  \text{ at the end of Phase 3 of the \reducecool protocol (\Cref{algorithm:reducecool}) }\}| \geq t + 1$. \label{item:retrievability}
     \end{compactitem}
    Assume a correct process $p_i$ obtains $(1, \omega^{(i)})$ from the \reducecool protocol. Hence, $v_i = 1$ at the end of the Phase 3 of the \reducecool protocol (\Cref{algorithm:reducecool}). %It means the variable $S_1$ verifies $|S_1| \geq 2t+1$ at line~\ref{line:reduce_cool_S1geq2tp1}.
By the retrievability property, a set $K$ of at least $t + 1$ correct processes $p_k$ has obtained $w^{(k)} \neq \phi$ and $s_k = 1$ at the end of the Phase 3 the \reducecool protocol (\Cref{algorithm:reducecool} and, due to non-duplicity, holds the same value $\bar{w}$, i.e., for every correct process $p_k \in K$, $w^{(k)} = \bar{w}$. 
Thus, for every correct process $p_l$ with $s_l = 0$, $p_l$ obtains a correctly-encoded RS symbol at line~\ref{line:majority} (as at most $t$ incorrect and at least $t + 1$ correct symbols are received by $p_l$). 
Therefore, every correct process that sends a symbol (line~\ref{line:reduce_cool_bcast_reconstruct_1} or line~\ref{line:reduce_cool_bcast_reconstruct_2}) does send a correctly-encoded RS symbol, which means that any correct process that decides at line~\ref{line:reduce_cool_decide_2_its} does decide the same value $\bar{w}$.
Moreover, $\bar{w}$ is proposed by a correct process due to the safety property of \reducecool.
    
    % \item Non-Duplicity is ensured by \cite[Lemma 3]{Chen2021extended}.
    % \item Retrievability is implied by~\cite[Lemma 4 (appendix G, equations 130 to 133)]{Chen2021extended}. 
    % \item Obligation is ensured by~\cite[Lemma 5 (appendix H)]{Chen2021extended}.
    
    % stating: "Assume that all honest processors have the same initial message as $\bar{w}_1$ [...] In Phase 3, all honest processors will again keep their success indicators as ones and keep their updated messages exactly the same as the initial message $\bar{w}_1$. In this scenario, the consensus of the votes $\{v_1, v_2, ... , v_n\}$ in Phase 3 should be $1$." The last sentence implies that for every correct process $p_i$, $v_i = 1$ by the end of Phase 3, because of the strong validity of the used binary consensus primitive. 
\end{compactitem}
As all properties are satisfied, the lemma holds.
\end{proof}

Then, we prove that our implementation satisfies strong validity.

\begin{theorem} [Strong validity]
\Cref{algorithm:gccool_protocol} satisfies strong validity.
\end{theorem}
\begin{proof}
By the obligation property of \reducecool, every correct process that proposes to the one-bit graded consensus primitive does so with $1$ (line~\ref{line:invoke_graded_consensus}).
This implies that every correct process that decides from the one-bit graded consensus primitive decides $(1, 1)$ (due to the strong validity property of the one-bit primitive).
Hence, every correct process that decides from \Cref{algorithm:gccool_protocol} does so with grade $1$ at line~\ref{line:decide_2_its}.
% Finally, Lemma~\ref{lemma:crucial_long_inputs_2} shows that there exists a unique value $\bar{w}$ such that (1) $\bar{w}$ is proposed by a correct process, and (2) every correct process that decides does decide $\bar{w}$, which concludes the proof.
Finally, there exists a unique value $\bar{w}$ such that, by \reducecool's safety (1) $\bar{w}$ is proposed by a correct process, and, due to the \reducecool's obligation property, (2) every correct process that decides does decide $\bar{w}$, which concludes the proof.
\end{proof}

Next, we prove external validity.

\begin{theorem} [External validity]
\Cref{algorithm:gccool_protocol} satisfies external validity.
\end{theorem}
\begin{proof}
If a correct process $p_i$ decides at line~\ref{line:decide_1_its}, the decision is valid as correct processes only propose valid values to graded consensus.
If a correct process $p_i$ decides $(\omega^{(i)}, g_i)$ at line~\ref{line:decide_2_its}, $v_j=1$ has been proposed to $\mathcal{GC}$ by some correct process $p_j$, due to the $\mathcal{GC}$'s safety property. Thus, the $\mathcal{R}_{\mathit{cool}}$'s consistency property implies that $\omega^{(i)} = \omega^{(j)}$. Moreover, the $\mathcal{R}_{\mathit{cool}}$'s safety property implies that $\omega^{j} = \omega_j$. Thus, $\omega^{(i)} = \omega_j$ is valid as correct processes only propose valid values to graded consensus.
%the strong value is valid due to Lemma~\ref{lemma:crucial_long_inputs_2}.
\end{proof}

The following theorem proves consistency.

\begin{theorem} [Consistency]
\Cref{algorithm:gccool_protocol} satisfies consistency.
\end{theorem}
\begin{proof}
If any correct process decides $(\bar{w}, 1)$ from \Cref{algorithm:gccool_protocol}, it does so at line~\ref{line:decide_2_its}.
Moreover, that implies that the process has previously decided $(1, 1)$ from the one-bit graded consensus primitive.
Therefore, due to the consistency property of the one-bit primitive, no correct process decides $(0, \cdot)$, which implies that any correct process that decides from \Cref{algorithm:gccool_protocol} necessarily does so at line~\ref{line:decide_2_its}.
Hence, every correct process that decides does decide value $\bar{w}$ due to $\mathcal{R}_{\mathit{cool}}$'s consistency property, which concludes the proof.
%Lemma~\ref{lemma:crucial_long_inputs_2}, which concludes the proof.
\end{proof}

Next, we prove integrity.

\begin{theorem} [Integrity]
\Cref{algorithm:gccool_protocol} satisfies integrity.
\end{theorem}
\begin{proof}
Integrity is satisfied since a process can only decide at line~\ref{line:decide_1_its} or at line~\ref{line:decide_2_its}.  %due to the $\mathit{decided}_i$ variable utilized at every correct process $p_i$.
% A correct process either decides at line~\ref{line:decide_1_its} or line~\ref{line:decide_3_its}. Moreover, due to the check at line~\ref{line:check_decided}, a correct process that has decided at line~\ref{line:decide_1_its} will never decide again at line~\ref{line:decide_3_its}.
\end{proof}

Finally, we prove termination.

\begin{theorem} [Termination]
\Cref{algorithm:gccool_protocol} satisfies termination.
\end{theorem}
\begin{proof}
Lemma~\ref{lemma:crucial_long_inputs} guarantees the termination of the \reducecool's instance executed at line~\ref{line:invoke_reduce}, while the termination of the binary graded consensus instance $\mathcal{GC}$ (executed at line~\ref{line:invoke_graded_consensus}) is ensured by the specification of the primitive. 
%Finally, the reconfiguration phase takes only constant number of rounds, which concludes the proof.
% \ayaz{I might be missing something, but is it possible that correct processes decide in different rounds? e.g. some decide at line~\ref{line:decide_1_its} and some decide at line~\ref{line:decide_3_its}. Right now the termination definition states that correct processes decide at the same round.} \jovan{Every correct process waits until the maximum possible time. I agree that this is a bit confusing; we should differentiate between deciding and terminating (this might be a bit cumbersome). For now, I removed the notion of ``simultaneous decision'' to avoid any confusion. We can reintroduce it for the real submission.}
\end{proof}

Finally, we prove the complexity of \Cref{algorithm:gccool_protocol}.

\begin{theorem} [Complexity]
In \Cref{algorithm:gccool_protocol}, every correct process sends 
$O\big( L + n \log(n) \big)$ bits.
Moreover, \Cref{algorithm:gccool_protocol} takes $7 \in O(1)$ rounds.
\end{theorem}
\begin{proof}
Each RS symbol is of size $O\big( \frac{L}{n} + \log(n) \big)$ bits.
Every correct process sends $4n$ RS symbols in \reducecool. %, a third RS symbol  at line~\ref{line:share_symbol}, and a fourth one at line~\ref{line:send_help_symbols}.
The other messages are sent in the execution of the binary graded consensus where each correct process broadcasts $2$ messages of 1 bit each (see~\cite{Lenzen2022}).
Hence, each correct process does send $O\big( L + n \log(n) \big)$ bits.
Lastly, the \reducecool protocol takes $5$ rounds to terminate, and the binary graded consensus takes $2$ rounds.% to terminate and the reconstruction phase takes $2$ additional rounds to terminate.
% (the round corresponding to line \ref{line:send_help_symbols} could be saved, since it corresponds to the first round of the \reducecool protocol).
\end{proof}
