# Supplementary material for: Efficient Signature-Free Validated Agreement
Source: arXiv:2403.08374 source file (2024-08-20)
Supplement: Supplementary file 2 [file nameopt_proof.tex]

\section{\nameopt: Formal Proof} \label{section:nameopt_proof}

In this section, we formally prove the correctness and complexity of \nameopt.
% Specifically, we first prove the correctness and complexity of \hashfin (\Cref{subsection:hashfin_proof}), a hash-based finisher primitive employed by \nameopt (see \Cref{subsection:hashfin}).
% Then, we provide \nameopt's proof.

%\input{appendix/hashfin}

%\subsection{\nameopt: Proof of Correctness \& Complexity} \label{subsection:nameopt_proof}

\noindent \textbf{Proof of correctness.}
We say that a correct process $p_i$ \emph{commits} a hash value $H$ in view $V \in [1, t + 1]$ if and only if $p_i$ invokes $\mathcal{F}.\mathsf{input}(\cdot, H)$ in view $V$ (line~\ref{line:commit_hash_value}).
Recall that if a correct process $p_i$ commits a hash value in some view $V < t + 1$, $p_i$ does not halt before it has completed view $V + 1$ (line~\ref{line:wait_for_completion}). 
We start by proving that if the first correct process commits a hash value $H$ in some view $V$, then all correct processes commit $H$ (and no other hash value) in view $V$ or $V + 1$ (given $V < t + 1$).

\begin{lemma} \label{lemma:first_commit}
Let $p_i$ be the first correct process to commit a hash value.
Let $p_i$ commit a hash value $H$ in view $V$.
Then, the following holds:
\begin{compactitem}
    \item If any correct process commits a hash value $H'$, then $H' = H$.

    \item If $V < t + 1$, then every correct process commits a hash value in view $V$ or $V + 1$.
\end{compactitem}
\end{lemma}
\begin{proof}
Recall that \nameopt ensures that each correct process $p_i$ commits at most one hash value (due to the $\mathit{committed\_view}_i$ variable).
As $p_i$ is the first correct process to commit a hash value, no correct process commits in any view smaller than $V$.
Moreover, if any correct process commits any hash value in view $V$, that hash value is $H$ due to the consistency property of $\mathcal{GC}_3$.

Let $V < t + 1$.
Consider now view $V + 1$.
Recall that $p_i$ (and any other correct process that has committed in view $V$) does not halt before completing view $V + 1$ (line~\ref{line:wait_for_completion}).
As $p_i$ has committed $H$ in view $V$, the consistency property of $\mathcal{GC}_3$ ensures that every correct process $p_k$ updates its $H_k$ variable to $H$ (Step 6).
Therefore, all correct processes propose $H$ to $\mathcal{GC}_1$ in view $V + 1$ (Step 1).
The strong validity property of $\mathcal{GC}_1$ guarantees that all correct processes decide $(H, 1)$ from $\mathcal{GC}_1$.
Thus, every correct process sends a $\langle \mathsf{HAPPY}, H \rangle$ message (Step 4).
This implies that every correct process $p_k$ updates its $\mathit{est}_k$ variable to $H$ (Step 4), and proposes $H$ to $\mathcal{GC}_3$ (Step 5).
Therefore, every correct process $p_k$ decides $(H, 1)$ from $\mathcal{GC}_3$ (due to the strong validity property of $\mathcal{GC}_3$).
Finally, every correct process $p_k$ commits $H$ in view $V + 1$ (Step 6), which concludes the proof.
\end{proof}

The following lemma proves that if a correct process decides $(H \neq \bot, \cdot)$ from $\mathcal{GC}_1$ in some view $V \in [2, t + 1]$, then a correct process has sent a $\langle \mathsf{HAPPY}, H \rangle$ message in view $V - 1$.

\begin{lemma} \label{lemma:decide_gc1_implies_happy}
If any correct process decides $(H \neq \bot, \cdot)$ from $\mathcal{GC}_1$ in any view $V \in [2, t + 1]$, then a correct process has sent a $\langle \mathsf{HAPPY}, H \rangle$ message in view $V - 1$.
\end{lemma}
\begin{proof}
Due to the safety property of $\mathcal{GC}_1$, a correct process has proposed $H$ to $\mathcal{GC}_1$, which implies that the process has decided $(H, \cdot)$ from $\mathcal{GC}_3$ in view $V - 1$ (Step 6).
The safety property of $\mathcal{GC}_3$ (in view $V - 1$) ensures that some correct process $p_k$ has proposed $H$ to $\mathcal{GC}_3$ in view $V - 1$. 
Thus, the value of the $\mathit{est}_k$ variable at process $p_k$ in view $V - 1$ was $H$, which implies that $p_k$ has received a $\langle \mathsf{HAPPY}, H \rangle$ message from $2t + 1$ processes in view $V - 1$.
As there are at most $t$ faulty processes, (at least) $t + 1$ of those messages are sent by correct processes, which concludes the proof.
\end{proof}

Next, we prove that if a correct process sends a $\mathsf{HAPPY}$ message for a hash value, the value that corresponds to that hash value is (1) known to at least \add{$t+1$ correct processes}, and (2) valid. %one correct process, and (2) valid.

\add{\begin{lemma} \label{lemma:happy_implies_awareness}
If a correct process sends a $\langle \mathsf{HAPPY}, H \rangle$ in some view $V$, then at least $t+1$ correct processes have set their respective $\mathit{known\_values}_{*}[H]$ variable to a value $v$ in some view $V' \leq V$, where $H = \mathsf{Hash}(v)$ and $\mathsf{valid}(v) = \mathit{true}$.
\end{lemma}
\begin{proof}
Let $p^*$ be the first correct process to ever send a $\langle \mathsf{HAPPY}, H \rangle$ message, for the given hash value $H$.
Let the aforementioned message by $p^*$ be sent in some view $V^*$.
To prove the lemma, it suffices to show that some set $S$ of $t+1$ correct processes have set their respective $\mathit{known\_values}_{*}[H]$ variable to a value $v$ in some view $V' \leq V^*$, where $H = \mathsf{Hash}(v)$ and $\mathsf{valid}(v) = \mathit{true}$.
We consider two scenarios:
\begin{compactitem}
    \item Let $p^*$ send the message at line~\ref{line:broadcast_happy_1}.
    In this case, $p^*$ has decided $(H \neq \bot, 1)$ from $\mathcal{GC}_1$ in view $V^*$.
    (Note that this implies that $V^* \in [2, t + 1]$.)
    Due to Lemma~\ref{lemma:decide_gc1_implies_happy}, there exists a correct process that has sent a $\mathsf{HAPPY}$ message for $H$ in view $V^* - 1$.
    This contradicts that the first $\mathsf{HAPPY}$ message from a correct process for $H$ is sent in view $V^*$.
    Therefore, this scenario is impossible.

    \item Let $p^*$ send the message at line~\ref{line:broadcast_happy_2}.
    In this case, $p^*$ has decided $(H, 1)$ from $\mathcal{GC}_2$ in view $V^*$.
    The awareness property of $\mathcal{GC}_2$ ensures that a set $S$ of $t+1$ correct processes have proposed $H$ to $\mathcal{GC}_2$.
    For each process $p_j \in S$, we further distinguish two possibilities:
    \begin{compactitem}
        \item Process $p_j$ has received $H$ from $\mathsf{leader}(V^*)$.
        % (This implies that $V^* \in [2, t + 1]$.)
        In this case, $H \in \mathit{accepted}_j[V^* - 1]$ (which implies $V^* \in [2, t + 1]$), which implies that $p_j$ has received a $\langle \mathsf{HAPPY}, H \rangle$ message from $t + 1$ processes in view $V^* - 1$.
        This contradicts the fact that the first $\mathsf{HAPPY}$ message from a correct process for $H$ is sent in view $V^*$.
        Hence, this case is impossible.

        \item Process $p_j$ has received a value $v$ from $\mathsf{leader}(V^*)$ such that $\mathsf{Hash}(v) = H$ and $\mathsf{valid}(v) = \mathit{true}$.
        In this case, the statement of the lemma is satisfied.
    \end{compactitem}
\end{compactitem}
As the statement of the lemma is satisfied in the only possible scenario, the lemma holds.
\end{proof}}

Let us denote by $\mathcal{V}$ the first view in which a correct process commits a hash value.
If such a view does not exist, $\mathcal{V} = \bot$.
Recall that Lemma~\ref{lemma:first_commit} proves that if $\mathcal{V} \neq \bot$, then all correct processes commit the same hash value, and they do so by the end of view $\mathcal{V} + 1$.
Let $\mathcal{H}$ denote the common hash value committed by correct processes; if $\mathcal{V} = \bot$, then $\mathcal{H} = \bot$.
Lastly, given that $\mathcal{V} \neq \bot$ (and $\mathcal{H} \neq \bot$), let $v^{\star}$ denote the value such that $\mathcal{H} = \mathsf{Hash}(v^{\star})$; 
%$\mathcal{H} = \mathsf{Merkle\_Root}(v^{\star})$; 
note that $v^{\star}$ is unique due to the collision-resistance of the hash function. %accumulator primitive.
The following lemma proves that if $\mathcal{V} \neq \bot$ (i.e., a correct process commits a hash value), then a correct process $p_i$ includes a value $v^{\star}$ in its $\mathit{known\_values}_i$ variable in a view smaller than or equal to $\mathcal{V}$.
% , where $\mathcal{H} = \mathsf{Merkle\_Root}(v)$.

% \begin{lemma} \label{lemma:committed_implies_known}
% Let $\mathcal{V} \neq \bot$.
% Then, there exists a correct process $p_i$ that sets its $\mathit{known\_values}_i[\mathcal{H}]$ variable to value $v^{\star}$ in a view $V \leq \mathcal{V}$.
% % in view $V \leq \mathcal{V}$, where $\mathcal{H} = \mathsf{Merkle\_Root}(v)$ and $\mathsf{valid}(v) = \mathit{true}$.
% \end{lemma}
% \begin{proof}
% As $\mathcal{H}$ is committed in view $\mathcal{V}$ by some correct process $p_i$, process $p_i$ has decided $(\mathcal{H}, 1)$ from $\mathcal{GC}_3$ in view $\mathcal{V}$.
% Therefore, the safety property of $\mathcal{GC}_3$ ensures that some correct process $p_j$ has proposed $\mathcal{H}$ to $\mathcal{GC}_3$.
% This implies that $\mathit{est}_j = \mathcal{H}$, which further proves that $p_j$ has received a $\mathsf{HAPPY}$ message for $\mathcal{H}$ in view $V^*$ from a correct process.
% Therefore, the lemma follows directly from Lemma~\ref{lemma:happy_implies_known}.
% \end{proof}

\add{\begin{lemma} \label{lemma:committed_implies_awareness}
Let $\mathcal{V} \neq \bot$.
Then, there exists a set $S$ of $t+1$ correct processes that set their respective $\mathit{known\_values}_{*}[\mathcal{H}]$ variable to value $v^{\star}$ in a view $V \leq \mathcal{V}$.
\end{lemma}
\begin{proof}
As $\mathcal{H}$ is committed in view $\mathcal{V}$ by some correct process $p_i$, process $p_i$ has decided $(\mathcal{H}, 1)$ from $\mathcal{GC}_3$ in view $\mathcal{V}$.
Therefore, the safety property of $\mathcal{GC}_3$ ensures that some correct process $p_j$ has proposed $\mathcal{H}$ to $\mathcal{GC}_3$.
This implies that $\mathit{est}_j = \mathcal{H}$, which further proves that $p_j$ has received a $\mathsf{HAPPY}$ message for $\mathcal{H}$ in view $V^*$ from a correct process.
Therefore, the lemma follows directly from Lemma~\ref{lemma:happy_implies_awareness}.
\end{proof}}

Next, we prove that value $v^{\star}$ is valid.

\begin{lemma} \label{lemma:valid_v_star}
Let $\mathcal{V} \neq \bot$.
Then, $\mathsf{valid}(v^{\star}) = \mathit{true}$.
\end{lemma}
\begin{proof}
As $\mathcal{V} \neq \bot$, Lemma~\ref{lemma:committed_implies_awareness} proves that a correct process $p_i$ sets its $\mathit{known\_values}_i[\mathcal{H}]$ variable to value $v^{\star}$ in some view $V \leq \mathcal{V}$.
Since process $p_i$ does so only upon checking the validity of $v^{\star}$ (line~\ref{line:check_validity_received_from_leader}), $v^{\star}$ is indeed valid.
\end{proof}

Next, we prove that all correct processes commit by the (end of the) first view with a correct leader.

\begin{lemma} \label{lemma:first_correct_leader}
Let $V \in [1, t + 1]$ denote the first view such that $\mathsf{leader}(V)$ is correct.
Then, all correct processes commit a hash value by the end of view $V$.
\end{lemma}
\begin{proof}
If there exists any correct process that commits in any view smaller than $V$, the lemma follows from Lemma~\ref{lemma:first_commit}.
Hence, let no correct process commit in any view smaller than $V$.
In this case, we distinguish two scenarios:
\begin{compactitem}
    \item There exists a correct process that decides $(H, 1)$ from $\mathcal{GC}_1$ in view $V$, for some hash value $H \neq \bot$.
    (This implies $V \in [2, t + 1]$.)
    Due to the safety property of $\mathcal{GC}_1$, there exists a correct process that has proposed $H$ to $\mathcal{GC}_1$, which implies that the process has decided $(H, \cdot)$ from $\mathcal{GC}_3$ in view $V - 1$.
    Therefore, the safety property of $\mathcal{GC}_3$ ensures that some correct process $p_j$ has previously proposed $H$ to $\mathcal{GC}_3$, which implies that $\mathit{est}_j = H$ in view $V - 1$.
    Hence, $p_j$ has received a $\langle \mathsf{HAPPY}, H \rangle$ message from $2t + 1$ processes in view $V - 1$, out of which at least $t + 1$ processes are correct.
    Thus, every correct process $p_k$ receives (at least) $t + 1$ $\langle \mathsf{HAPPY}, H \rangle$ messages in view $V - 1$, which implies that $H \in \mathit{accepted}_k[V - 1]$.
    % Thus, $H \in \mathit{accepted}_k[V - 1]$, for every correct process $p_k$.

    Due to the consistency property of $\mathcal{GC}_1$, the leader decides $(H, \cdot)$ from $\mathcal{GC}_1$.
    Therefore, the leader broadcasts $H$ (Step 2 of view $V$), which implies that all correct processes propose $H$ to $\mathcal{GC}_2$ (recall that $H$ is accepted at all correct processes).
    Moreover, the strong validity property of $\mathcal{GC}_2$ ensures that all correct processes decide $(H, 1)$ from $\mathcal{GC}_2$.
    Thus, all correct processes broadcast a $\mathsf{HAPPY}$ message for $H$ in view $V$ (Step 4), which implies that every correct process $p_k$ updates its $\mathit{est}_k$ variable to $H$ (Step 4).
    This further means that all correct processes propose $H$ to $\mathcal{GC}_3$ (Step 5).
    Finally, all correct processes decide $(H, 1)$ from $\mathcal{GC}_3$ (due to its strong validity property), which concludes the proof in this case.

    \item No correct process decides $(\cdot, 1)$ from $\mathcal{GC}_1$ in view $V$.
    We further distinguish two cases:
    \begin{compactitem}
        \item The leader decides $(H, 0)$ from $\mathcal{GC}_1$ in view $V$, for some hash value $H \neq \bot$.
        Due to the safety property of $\mathcal{GC}_1$, there exists a correct process that has proposed $H$ to $\mathcal{GC}_1$, which implies that the process has decided $(H, \cdot)$ from $\mathcal{GC}_3$ in view $V - 1$.
        Therefore, the safety property of $\mathcal{GC}_3$ ensures that some correct process $p_j$ has previously proposed $H$ to $\mathcal{GC}_3$, which implies that $\mathit{est}_j = H$ in view $V - 1$.
        Hence, $p_j$ has received a $\langle \mathsf{HAPPY}, H \rangle$ message from $2t + 1$ processes in view $V - 1$, out of which (at least) $t + 1$ are correct.
        Thus, $H \in \mathit{accepted}_k[V - 1]$, for every correct process $p_k$.

        In this case, the leader broadcasts $H$ (Step 2 of view $V$), which implies that all correct processes propose $H$ to $\mathcal{GC}_2$ (recall that $H$ is accepted at all correct processes).
        Moreover, the strong validity property of $\mathcal{GC}_2$ ensures that all correct processes decide $(H, 1)$ from $\mathcal{GC}_2$.
        Thus, all correct processes broadcast a $\mathsf{HAPPY}$ message for $H$ in view $V$ (Step 4), which implies that every correct process $p_k$ updates its $\mathit{est}_k$ variable to $H$ (Step 4) and proposes $H$ to $\mathcal{GC}_3$ (Step 5).
        Finally, all correct processes decide $(H, 1)$ from $\mathcal{GC}_3$ (due to its strong validity property), which concludes the proof in this case.

        \item The leader decides $(\bot, \cdot)$ from $\mathcal{GC}_1$.
        Hence, the leader broadcasts its value $v$ (Step 2 of view $V$), which implies that all correct processes propose $H = \mathsf{Hash}(v)$ to $\mathcal{GC}_2$. %$H = \mathsf{Merkle\_Root}(v)$ to $\mathcal{GC}_2$.
        Moreover, the strong validity property of $\mathcal{GC}_2$ ensures that all correct processes decide $(H, 1)$ from $\mathcal{GC}_2$.
        Thus, all correct processes broadcast a $\mathsf{HAPPY}$ message for $H$ in view $V$ (Step 4), which implies that every correct process $p_k$ updates its $\mathit{est}_k$ variable to $H$ (Step 4) and proposes $H$ to $\mathcal{GC}_3$ (Step 5).
        Lastly, all correct processes decide $(H, 1)$ from $\mathcal{GC}_3$ (due to its strong validity property), which concludes the proof in this case as well.
    \end{compactitem}
\end{compactitem}
The lemma holds as its statement is satisfied in all possible scenarios.
\end{proof}

We are ready to prove that $\mathcal{V} \neq \bot$. 
Concretely, we prove that $\mathcal{V} \in [1, f + 1]$.

\begin{lemma} \label{lemma:commit_eventually_occurs}
$\mathcal{V} \in [1, f + 1]$.
\end{lemma}
\begin{proof}
Recall that $f \leq t$.
Hence, there exists a view with a correct leader.
Let $V$ be the first such view.
Lemma~\ref{lemma:first_correct_leader} proves that $\mathcal{V} \leq V$.
As $V \in [1, f + 1]$, the lemma holds.
\end{proof}

We are ready to prove that \nameopt ensures that all required assumptions of $\mathcal{F}$ are ensured.

\begin{lemma} \label{lemma:required_assumptions_satisfied}
\nameopt (\Cref{algorithm:optimal_2}) ensures that all assumptions required by $\mathcal{F}$ are satisfied.
\end{lemma}
\begin{proof}
All correct processes input a pair to $\mathcal{F}$ as all correct processes commit a hash value due to lemmas~\ref{lemma:first_commit},~\ref{lemma:first_correct_leader} and~\ref{lemma:commit_eventually_occurs}.
No correct process halts unless it has previously output a value from $\mathcal{F}$ as a correct process $p_i$ halts (line~\ref{line:halt_optimal_2}) only after it has output a value from $\mathcal{F}$ (line~\ref{line:upon_output_optimal_2}).
Recall that all correct processes commit the same hash value $\mathcal{H}$ (by Lemma~\ref{lemma:first_commit}).
% This, along with the fact that the $\mathsf{Merkle\_Root}(\cdot)$ function is collision-resistant, implies that there exists a unique value $v^{\star}$ such that $\mathsf{Merkle\_Root}(\mathcal{H}) = v^{\star}$.
Moreover, the following holds for value $v^{\star}$:
\begin{compactitem}
    \item At least $t+1$ correct processes input $(v^{\star} \neq \bot, \cdot)$ to $\mathcal{F}$.
    As no correct process inputs a pair to $\mathcal{F}$ before view $\mathcal{V}$ (due to the definition of view $\mathcal{V}$) and there exists at least $t+1$ correct processes that set their respective $\mathit{known\_values}_{*}[\mathcal{H}]$ variables to value $v^{\star}$ in view $V \leq \mathcal{V}$ (by Lemma~\ref{lemma:valid_v_star}), these $t+1$ correct processes are guaranteed to input $v^{\star}$ to $\mathcal{F}$ (line~\ref{line:commit_hash_value}).
    
    %one correct process $p_i$ that sets its $\mathit{known\_values}_i[\mathcal{H}]$ variable to value $v^{\star}$ in view $V \leq \mathcal{V}$ (by Lemma~\ref{lemma:happy_implies_known}), this correct process is guaranteed to input $v^{\star}$ to $\mathcal{F}$ (line~\ref{line:commit_hash_value}).

    \item If any correct process inputs $(v \neq \bot, \cdot)$, then $v = v^{\star}$ because (1) all correct processes commit the same hash value $\mathcal{H}$ such that $\mathcal{H} = \mathsf{Hash}(v^{\star})$, %$\mathcal{H} = \mathsf{Merkle\_Root}(v^{\star})$,
    (2) all correct processes input a value $v$ with $\mathcal{H} = \mathsf{Merkle\_Root}(v)$, %$\mathcal{H} = \mathsf{Merkle\_Root}(v)$,
    and (3) the $\mathsf{Hash}(\cdot)$ function is collision-resistant. %$\mathsf{Merkle\_Root}(\cdot)$ function is collision-resistant.
    The argument above ensures that any value $v \neq \bot$ input to $\mathcal{F}$ must equal $v^{\star}$.

    \item If any correct process inputs $(\cdot, H)$, then $H = \mathsf{Hash}(v^{\star})$ because (1) $H = \mathcal{H}$, and (2) $\mathcal{H} = \mathsf{Hash}(v^{\star})$. % \item If any correct process inputs $(\cdot, H)$, then $H = \mathsf{Merkle\_Root}(v^{\star})$ because (1) $H = \mathcal{H}$, and (2) $\mathcal{H} = \mathsf{Merkle\_Root}(v^{\star})$.
\end{compactitem}
As all assumptions required by $\mathcal{F}$ are satisfied, the lemma holds.
\end{proof}

% We denote by $v^{\star}$ the value for which $\mathcal{H} = \mathsf{Merkle\_Root}(v^{\star})$ (as in \Cref{subsection:hashfin}).
% The following theorem proves \nameopt's agreement property.

% The following lemma proves that all correct processes decide value $v^{\star}$ from \n
% ameopt.
The following theorem proves the correctness of \nameopt.

\begin{theorem} [Correctness]
\nameopt (\Cref{algorithm:optimal_2}) is correct, i.e., it satisfies agreement, external validity and termination.
\end{theorem}
\begin{proof}
Lemma~\ref{lemma:required_assumptions_satisfied} proves that $\mathcal{F}$ behaves according to its specification.
Therefore, the safety property of $\mathcal{F}$ ensures that correct processes only output $v^{\star}$ from $\mathcal{F}$, thus proving the agreement property of \nameopt.
Similarly, the liveness property of $\mathcal{F}$ ensures that all correct processes eventually output from $\mathcal{F}$, thus showing the termination property of \nameopt.
Finally, the external validity property of \nameopt follows from Lemma~\ref{lemma:valid_v_star}.
\end{proof}

% \begin{theorem} [Agreement]
% \nameopt (\Cref{algorithm:optimal_2}) satisfies agreement.
% \end{theorem}
% \begin{proof}
% Lemma~\ref{lemma:required_assumptions_satisfied} proves that $\mathcal{F}$ behaves according to its specification (see \Cref{subsection:hashfin}).
% Thus, the safety property of $\mathcal{F}$ ensures that all correct processes that decide from \nameopt decide value $v^{\star}$.
% \end{proof}

% Next, we prove that \nameopt satisfies external validity.

% \begin{theorem} [External validity]
% \nameopt (\Cref{algorithm:optimal_2}) satisfies external validity.
% \end{theorem}
% \begin{proof}
% Lemma~\ref{lemma:required_assumptions_satisfied} proves that $\mathcal{F}$ behaves according to its specification (see \Cref{subsection:hashfin}).
% Thus, the safety property of $\mathcal{F}$ ensures that all correct processes that decide do so with value $v^{\star}$.
% Moreover, Lemma~\ref{lemma:committed_implies_known} guarantees that $v^{\star}$ is valid.
% \end{proof}

% Finally, we prove the termination property of \nameopt.

% \begin{theorem} [Termination]
% \nameopt (\Cref{algorithm:optimal_2}) satisfies termination.
% \end{theorem}
% \begin{proof}
% Lemma~\ref{lemma:required_assumptions_satisfied} proves that $\mathcal{F}$ behaves according to its specification (see \Cref{subsection:hashfin}).
% Therefore, the termination property of \nameopt follows from the liveness property of $\mathcal{F}$.
% \end{proof}

\medskip
\noindent \textbf{Proof of complexity.}
First, we show that any non-leader correct process sends $O(n\kappa)$ bits in a view.

\begin{lemma} \label{lemma:non_leader_bits}
Consider any correct process $p_i$ and any view $V$ such that $\mathsf{leader}(V) \neq p_i$.
Then, $p_i$ sends $O(n\kappa)$ bits in $V$.
\end{lemma}
\begin{proof}
Process $p_i$ sends $O(n\kappa)$ bits while executing $\mathcal{GC}_1$, $\mathcal{GC}_2$ and $\mathcal{GC}_3$.
Moreover, process $p_i$ sends $O(n\kappa)$ bits via $\mathsf{HAPPY}$ messages.
Finally, process $p_i$ sends $O(n)$ bits via $\mathsf{SAD}$ messages.
Hence, $p_i$ sends $O(n\kappa) + O(n) = O(n\kappa)$ bits in $V$.
\end{proof}

Next, we prove that a correct leader sends $O(nL + n\kappa)$ bits in a view.

\begin{lemma} \label{lemma:leader_bits}
Consider any correct process $p_i$ and any view $V$ such that $\mathsf{leader}(V) = p_i$.
Then, $p_i$ sends $O(nL + n\kappa)$ bits in $V$.
\end{lemma}
\begin{proof}
Process $p_i$ sends $O(n\kappa)$ bits while executing $\mathcal{GC}_1$, $\mathcal{GC}_2$ and $\mathcal{GC}_3$.
Moreover, process $p_i$ sends $O(n\kappa)$ bits via $\mathsf{HAPPY}$ and $\mathsf{SAD}$ messages.
Finally, process $p_i$ sends $O(nL + n\kappa)$ bits in Step 2 of $V$.
Thus, $p_i$ sends $O(n\kappa) + O(nL + n\kappa) = O(nL + n\kappa)$ bits in $V$.
\end{proof}

Next, we prove that no correct process enters any view greater than $\min(t + 1, \mathcal{V} + 2)$.

\begin{lemma} \label{lemma:views_entered}
No correct process enters any view greater than $\min(t + 1, \mathcal{V} + 2)$.
\end{lemma}
\begin{proof}
If $\mathcal{V} + 3 > t + 1$, the lemma trivially holds.
Otherwise, Lemma~\ref{lemma:first_commit} proves that all correct processes commit a hash value by (the end of) view $\mathcal{V} + 1$.
As any correct process that commits a hash value in some view $V$ only enters the next view $V + 1$, no correct process enters any view greater than $\mathcal{V} + 2$.
\end{proof}

The following theorem proves that $\min(t + 1, \mathcal{V} + 2) \in O(f)$.

\begin{lemma} \label{lemma:min_o_f}
$\min(t + 1, \mathcal{V} + 2) \in O(f)$.    
\end{lemma}
\begin{proof}
By Lemma~\ref{lemma:commit_eventually_occurs}, $\mathcal{V} \in O(f)$.
If $t + 1 \leq \mathcal{V} + 2$, $\mathcal{V} \in \{t - 1, t, t + 1\}$.
Therefore, $\min(t + 1, \mathcal{V} + 2) = t + 1 \in O(f)$.
If $t + 1 > \mathcal{V} + 2$, then $\min(t + 1, \mathcal{V} + 2) = \mathcal{V} + 2 \in O(f)$.
\end{proof}

We are ready to prove the bit complexity of \nameopt.

\begin{theorem} [Bit complexity]
\nameopt (\Cref{algorithm:optimal_2}) achieves $O(nL + n^2 (f + 1) \kappa)$ bit complexity.%$O(nL + n^2 (f + \log n) \kappa)$ bit complexity.
\end{theorem}
\begin{proof}
Lemma~\ref{lemma:first_correct_leader} proves that, for every view $V \in [1, \mathcal{V} - 1]$, $\mathsf{leader}(V)$ is faulty.
Moreover, Lemma~\ref{lemma:views_entered} shows that no correct process enters any view greater than $\min(t + 1, \mathcal{V} + 2)$.
Lastly, Lemma~\ref{lemma:min_o_f} proves that $\min(t + 1, \mathcal{V} + 2) \in O(f)$.
Hence, in every view $V \in [1, \mathcal{V} - 1]$, each correct process sends $O(n\kappa)$ bits (by \Cref{lemma:non_leader_bits}).
Moreover, in every view $V \in [\mathcal{V}, \min(t + 1, \mathcal{V} + 2)]$, (1) $\mathsf{leader}(V)$ (if correct) sends $O(nL + n\kappa)$ bits (by \Cref{lemma:leader_bits}), and (2) every other correct process sends $O(n\kappa)$ bits (by \Cref{lemma:non_leader_bits}).
Therefore, while executing views $[1, \min(t + 1, \mathcal{V} + 2)]$, correct process send $f \cdot n \cdot O(n\kappa) + O(1) \cdot \big( O(nL + n\kappa) + n \cdot O(n\kappa) \big) = O(n^2 f \kappa) + O(nL + n\kappa) + O(n^2\kappa) = O(nL + n^2 f \kappa)$ bits.
Moreover, correct processes exchange $O(nL + n^2\log(n))$ bits while executing $\mathcal{F}$. %$O(nL + n^2\log(n)\kappa)$ bits while executing $\mathcal{F}$.
Therefore, the bit complexity of \nameopt is $O(nL + n^2 f \kappa) + O(nL + n^2\kappa) = O(nL + n^2(f + 1) \kappa)$. %$O(nL + n^2 f \kappa) + O(nL + n^2\log(n)\kappa) = O(nL + n^2(f + \log n) \kappa)$.
\end{proof}

Finally, we prove that \nameopt achieves early stopping.

\begin{theorem} [Early stopping]
\nameopt (\Cref{algorithm:optimal_2}) achieves early stopping.
\end{theorem}
\begin{proof}
By Lemma~\ref{lemma:first_commit}, all correct processes start $\mathcal{F}$ by the end of $\mathcal{V} + 1$ view.
Therefore, Lemma~\ref{lemma:commit_eventually_occurs} proves that all correct processes start executing $\mathcal{F}$ in $O(f)$ time.
The liveness property of $\mathcal{F}$ ensures that all correct processes output a value in $O(f) + 2\delta \in O(f)$ time.
Finally, given that each view of \nameopt takes only $O(1)$ time, the proof is concluded.
\end{proof}
